# Supplementary material for: Effects of particle roughness on the rheology and structure of capillary suspensions
Source: arXiv:2203.07779 source file (2022-05-11)
Supplement: Supplementary file 1 [file Supplemental_Information.pdf]

# Supplementary Information for Effects of particle roughness on the rheology and structure of capillary suspensions

Jens Allard[a,*], Sanne Burgers[a,1], Miriam Candelaria Rodríguez González[b], Yanshen Zhu[a], Steven De Feyter[b], Erin Koos[a]

[a] KU Leuven, Chemical Engineering Department, Celestijnenlaan 200J, Leuven, 3001, Belgium
[b] KU Leuven, Department of Chemistry, Celestijnenlaan 200F, Leuven, 3001, Belgium
[1] Present address: Rijksweg 12, 2870 Puurs, Belgium
[*] E-mail: jens.allard@kuleuven.be

## List of Figures

S1 Frequency sweep of a smooth particle capillary suspension . . . 2
S2 Frequency sweeps at different gaps and Normal force during loading of a smooth particle capillary suspension . . . 2
S3 Confocal micrograph of the particle channel . . . 3
S4 Amplitude sweeps and corresponding confocal micrographs of capillary suspensions with particles of different roughness . . . 4
S5 Amplitude sweeps performed on a rheometer mounted to a confocal microscope . . . 5
S6 Larger scale images of a smooth particle capillary suspension . . . 6
S7 Larger scale images of an R250 particle capillary suspension . . . 7
S8 Example fit of the third harmonic elastic and viscous stress scalings in the asymptotically nonlinear regime . . . 7
S9 All forward and backward amplitude sweeps for the MAOS protocol . . . 8

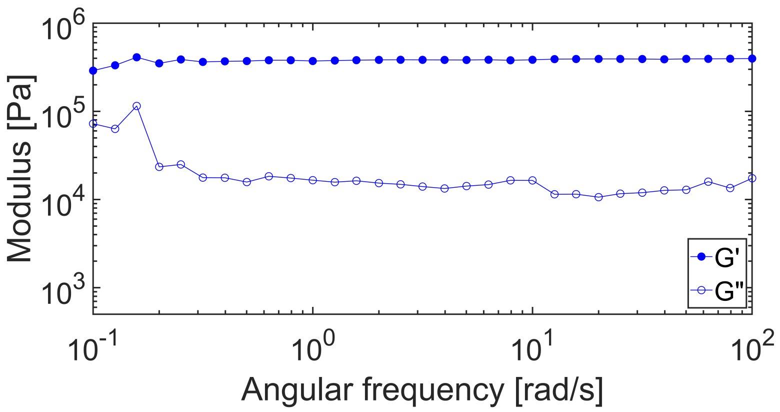


Figure S1: Frequency sweep of a smooth particle capillary suspension with $\phi_{\text{solid}} = 20$ vol%, $\phi_{\text{sec}} = 1$ vol%

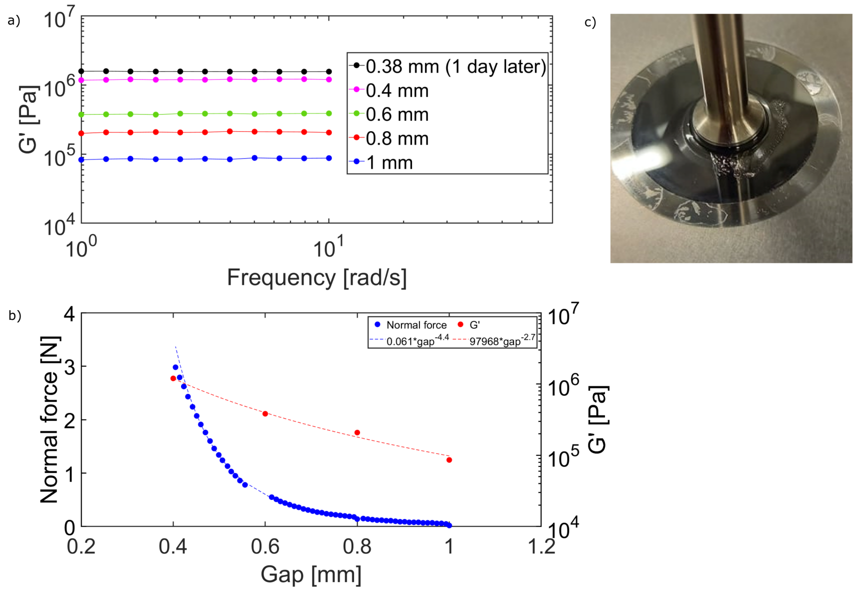


Figure S2: a) Frequency sweeps at different gaps of a smooth particle capillary suspension with 10 $\mu$m particles and $\phi_{\text{solid}} = 20$ vol%, $\phi_{\text{sec}} = 1$ vol%. b) Normal force during loading phase and frequency sweep data from a) versus measurement gap. c) Picture of the sample at 0.4 mm gap showing the transparent bulk liquid was pushed out of the measurement gap

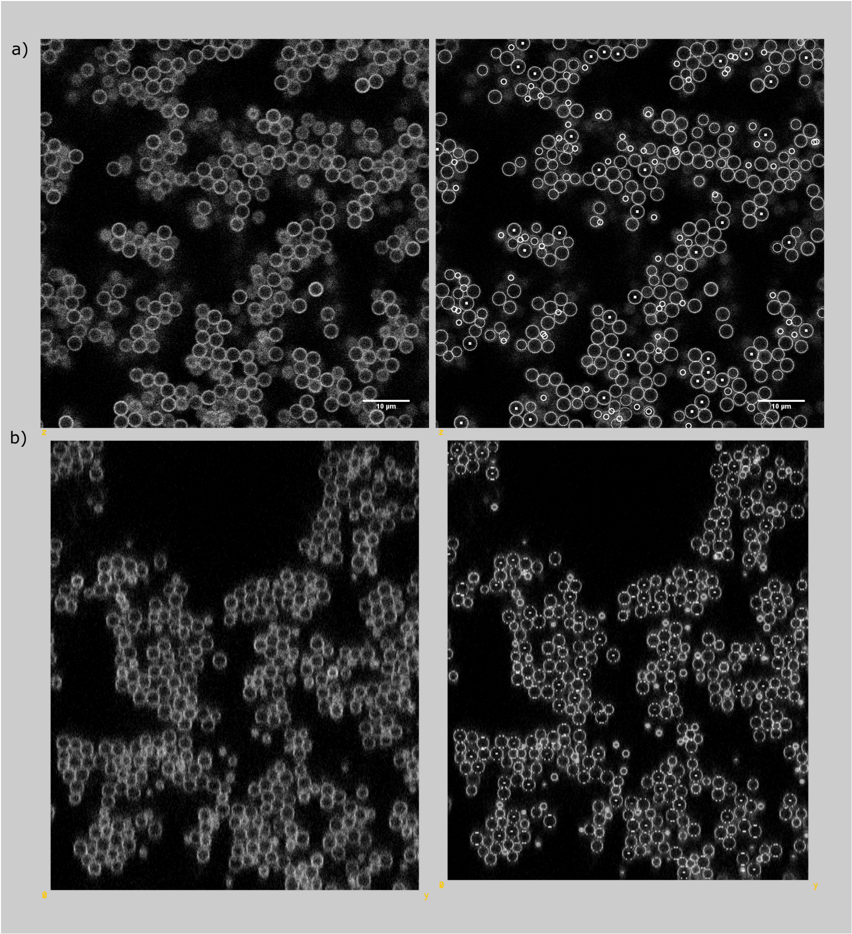


Figure S3: a) Confocal micrograph of the particle channel (XY-plane) and corresponding detection image for a smooth particle capillary suspension b) YZ-plane confocal micrograph of the particle channel reconstructed from the 300 XY images and corresponding detection image

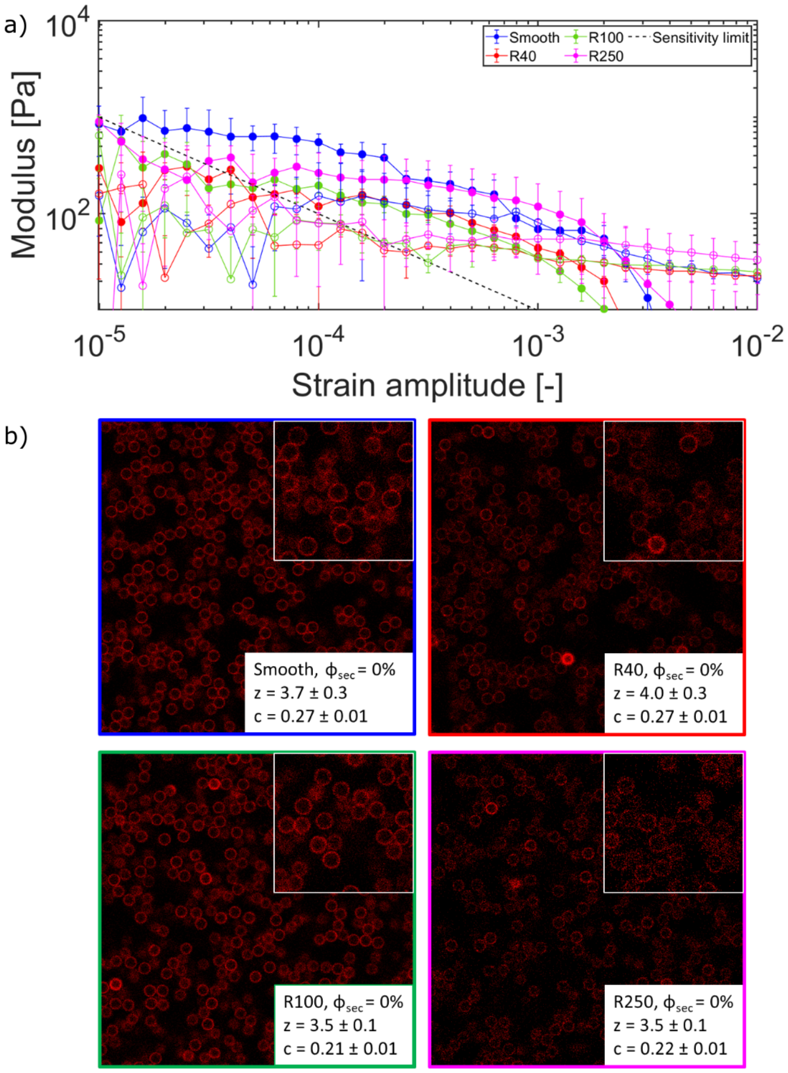


Figure S4: a) Amplitude sweeps and b) corresponding confocal micrographs of capillary suspensions with particles of different roughness and $\phi_{\text{solid}} = 20$ vol%, $\phi_{\text{sec}} = 0$ vol%. Filled symbols: $G'$, open symbols: $G''$. The dotted line shows the sensitivity limit calculated from the low torque limit provided by the manufacturer. Confocal micrographs in b) have a dimension of 82 $\mu$m x 82 $\mu$m. The particles are shown as red rings. Insets show a magnified image.

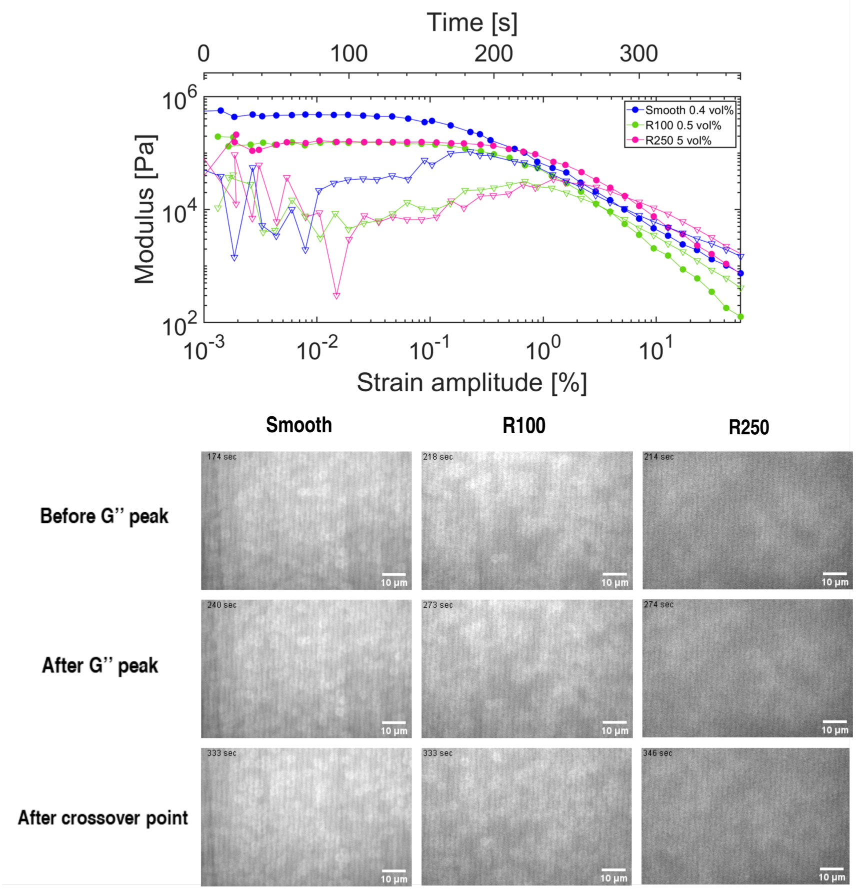


Figure S5: Amplitude sweeps performed on a rheometer mounted to a confocal microscope. Each curve has the corresponding micrographs of the particle detection channel and a supplemental video (1-3) both imaged at the plane below the oscillating top plate. The smooth particle suspension already shows local particle rearrangement around the $G''$ peak. Filled symbols: $G'$, open symbols: $G''$

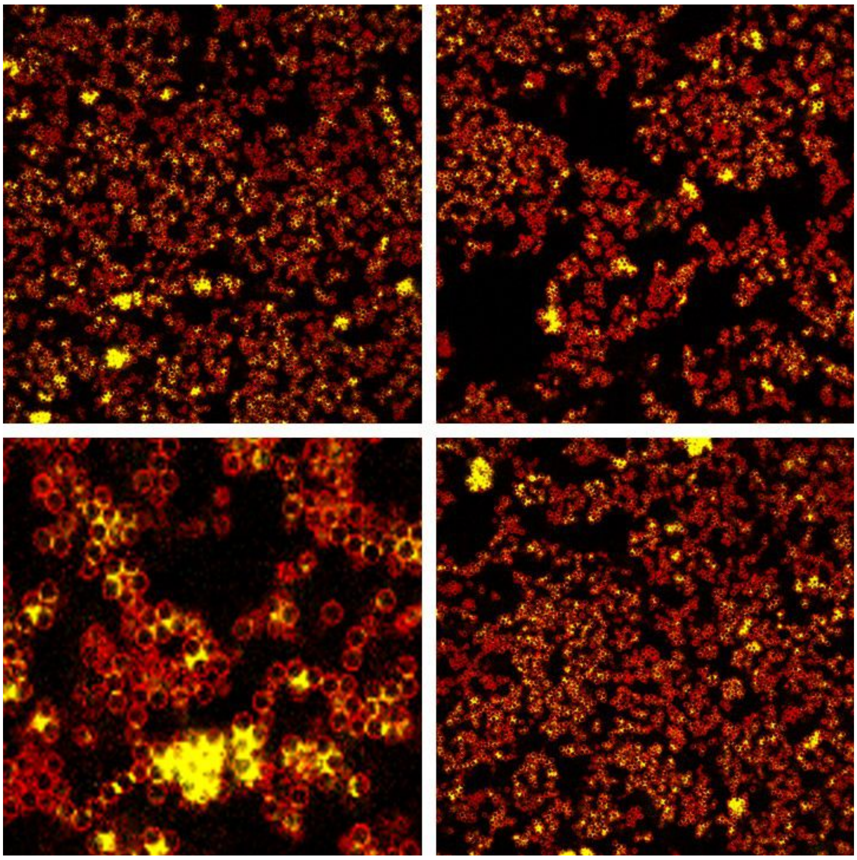

Figure S6: Larger scale images (246 $\mu$m x 246 $\mu$m) of a smooth particle capillary suspension with $\phi_{\text{solid}} = 20$ vol%, $\phi_{\text{sec}} = 1$ vol%

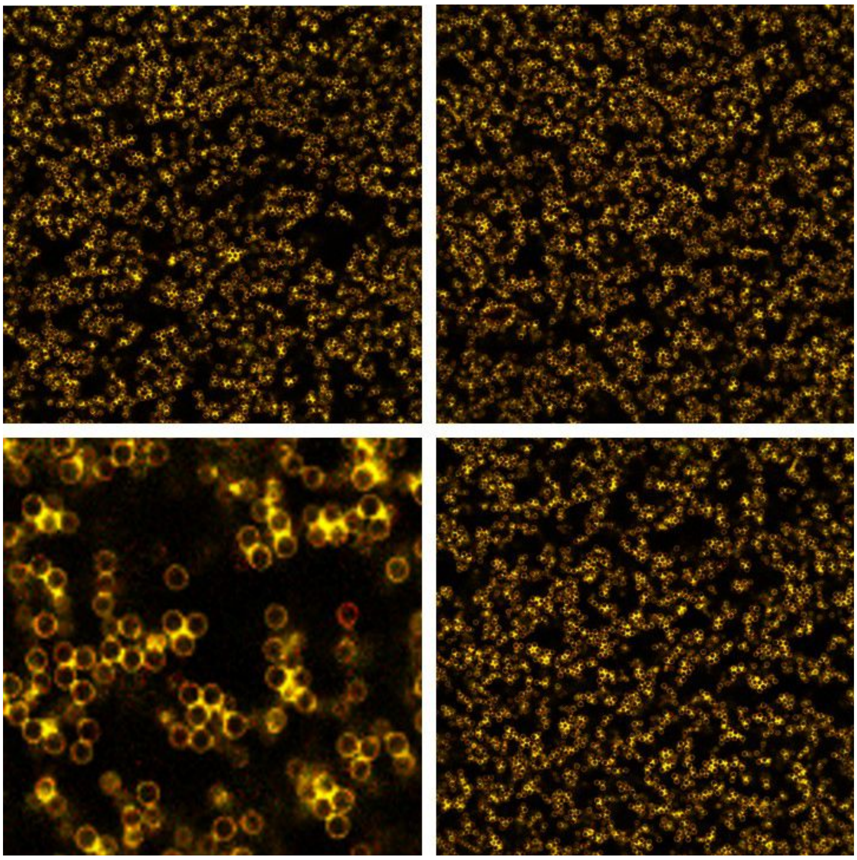

Figure S7: Larger scale images (246 $\mu$m x 246 $\mu$m) of an R250 particle capillary suspension with $\phi_{\text{solid}} = 20$ vol%, $\phi_{\text{sec}} = 5$ vol%

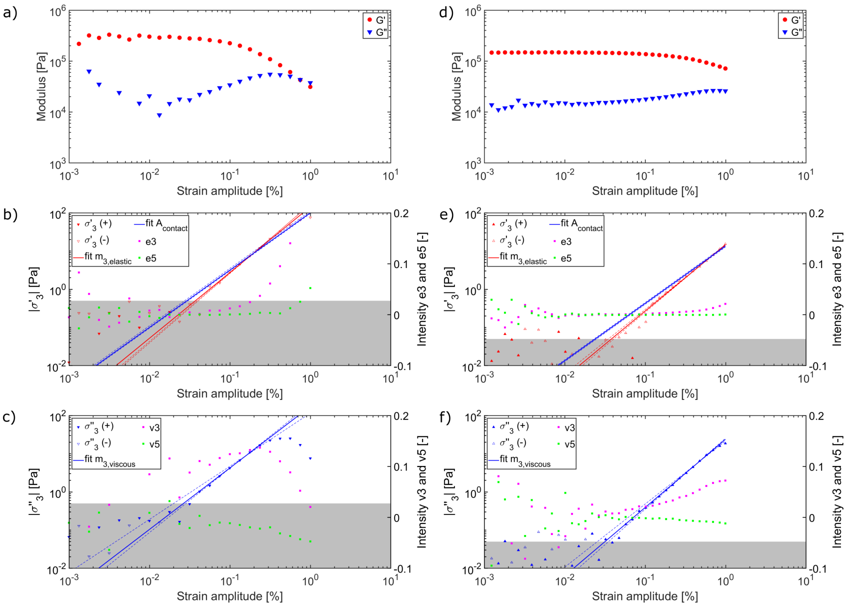


Figure S8: Example fit of the third harmonic elastic and viscous stress scalings in the asymptotically nonlinear regime for measurements on an R250 sample with an (a-c) 8 mm and (d-f) 25 mm parallel plate geometry. The stress noise floor is shown as gray shading below 0.5 Pa and 0.05 Pa, respectively. The dashed lines show the sensitivity of the fits by including or excluding an extra data point. The second Y-axis shows the relative magnitude of the third and fifth harmonic normalized by the first harmonic.

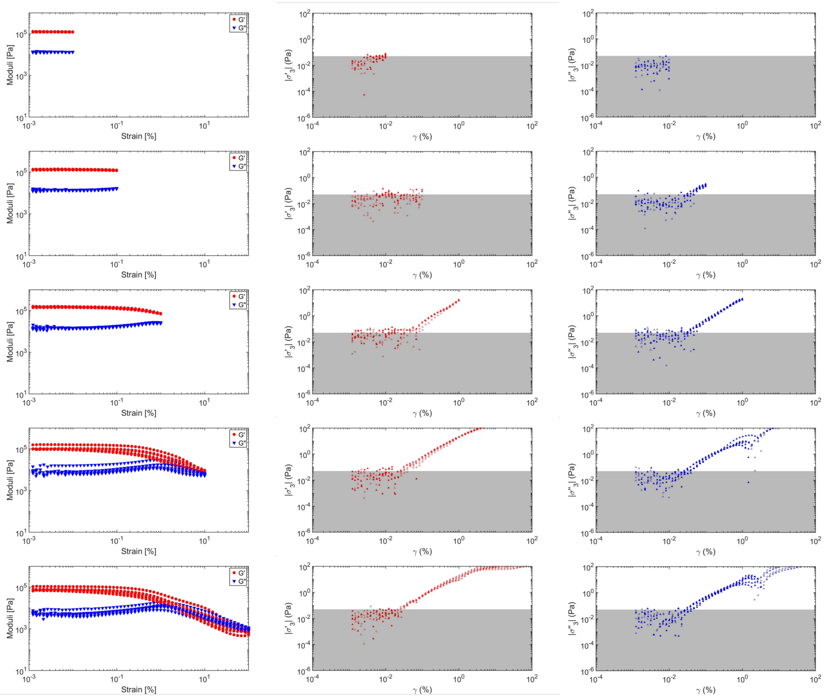


Figure S9: All forward and backward amplitude sweeps for the MAOS protocol measured on an R250 sample with a 25 mm parallel plate geometry. The stress noise floor is shown as gray shading below 0.05 Pa. Up until a maximum strain of 1 %, the moduli obtained with forward and backward sweeps overlap completely, indicating reversible behavior.
